# Supplementary material for: Chained Multi-stream Networks Exploiting Pose, Motion, and Appearance for Action Classification and Detection
Source: arXiv:1704.00616 source file (2017-05-26)
Supplement: Supplementary file 1 [file sup_mat.tex]

\section{Network inputs}

Figures \ref{fig:NetworkInputs1} and \ref{fig:NetworkInputs2} show sample frames of network inputs on different actions from J-HMDB \cite{JhmdbDataset}, UCF101 \cite{UCF101}, and HMDB51 \cite{HMDB51} datasets. 

  %---- Figure: Pre-processing and tube extraction

 \begin{figure}[t!]
 \centering
    \subfloat{%  
        \includegraphics[height=.4\linewidth,width=.75\linewidth]{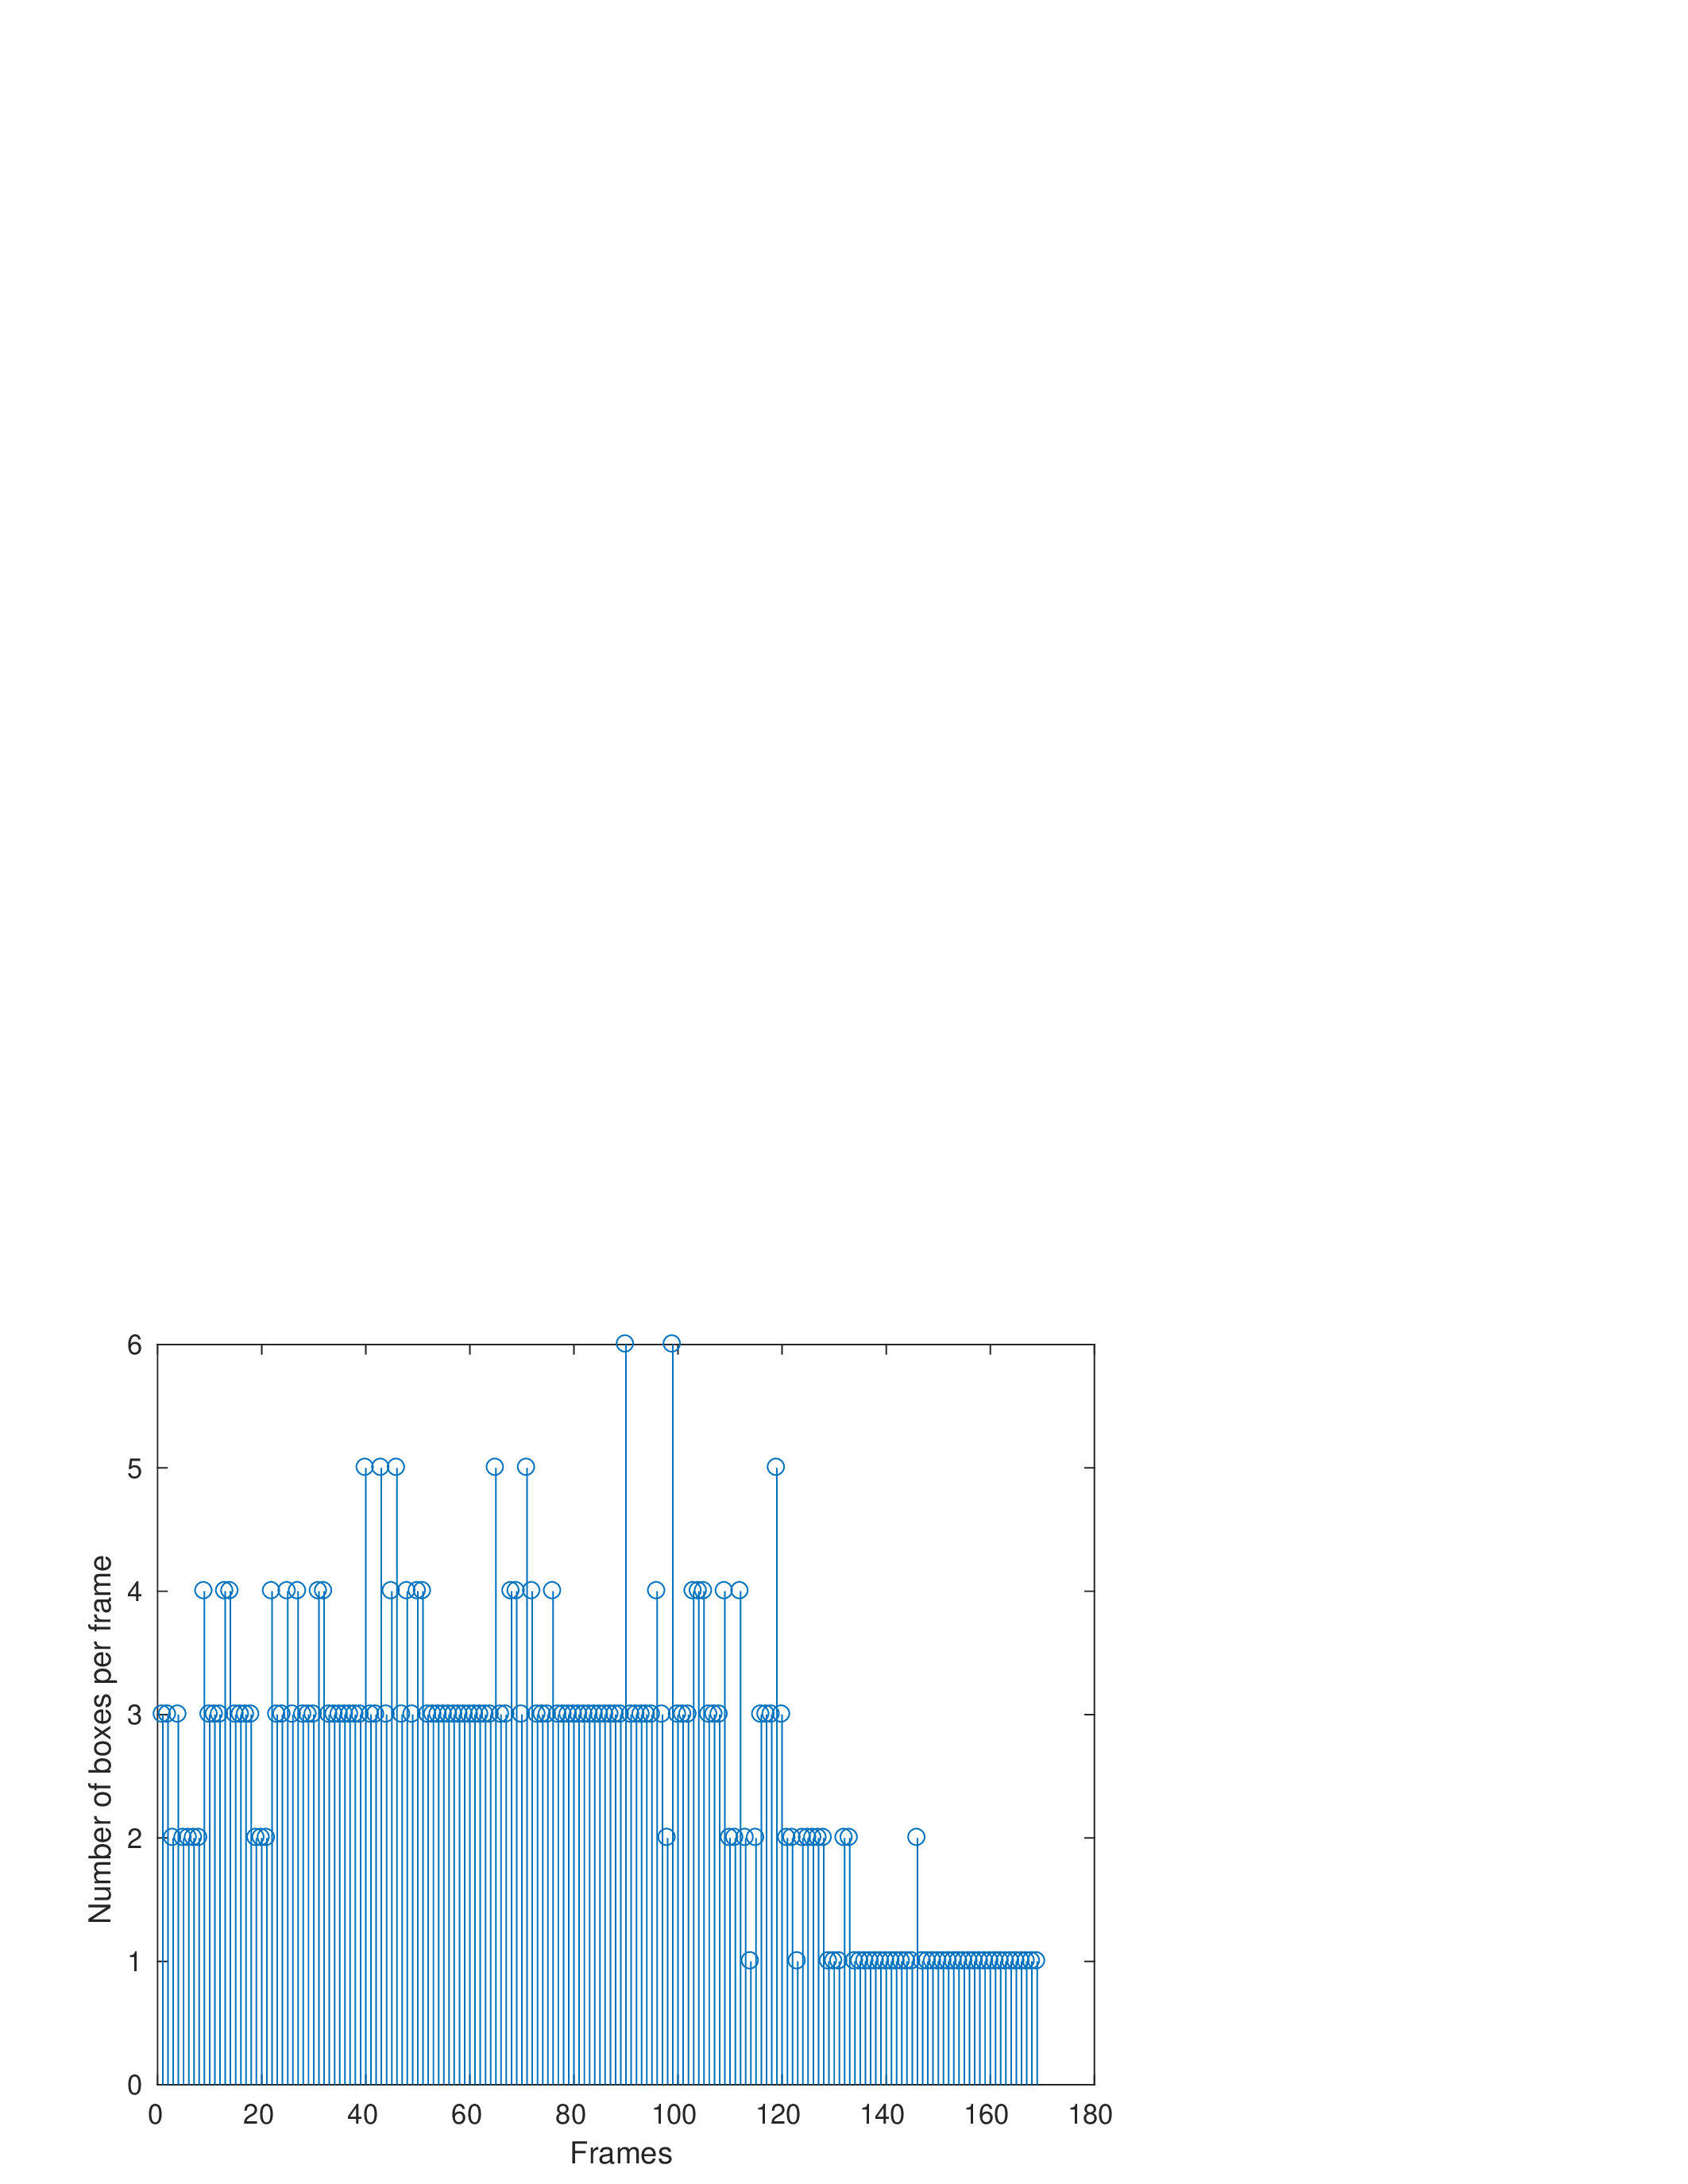}
       % \includegraphics[width=.3\linewidth]{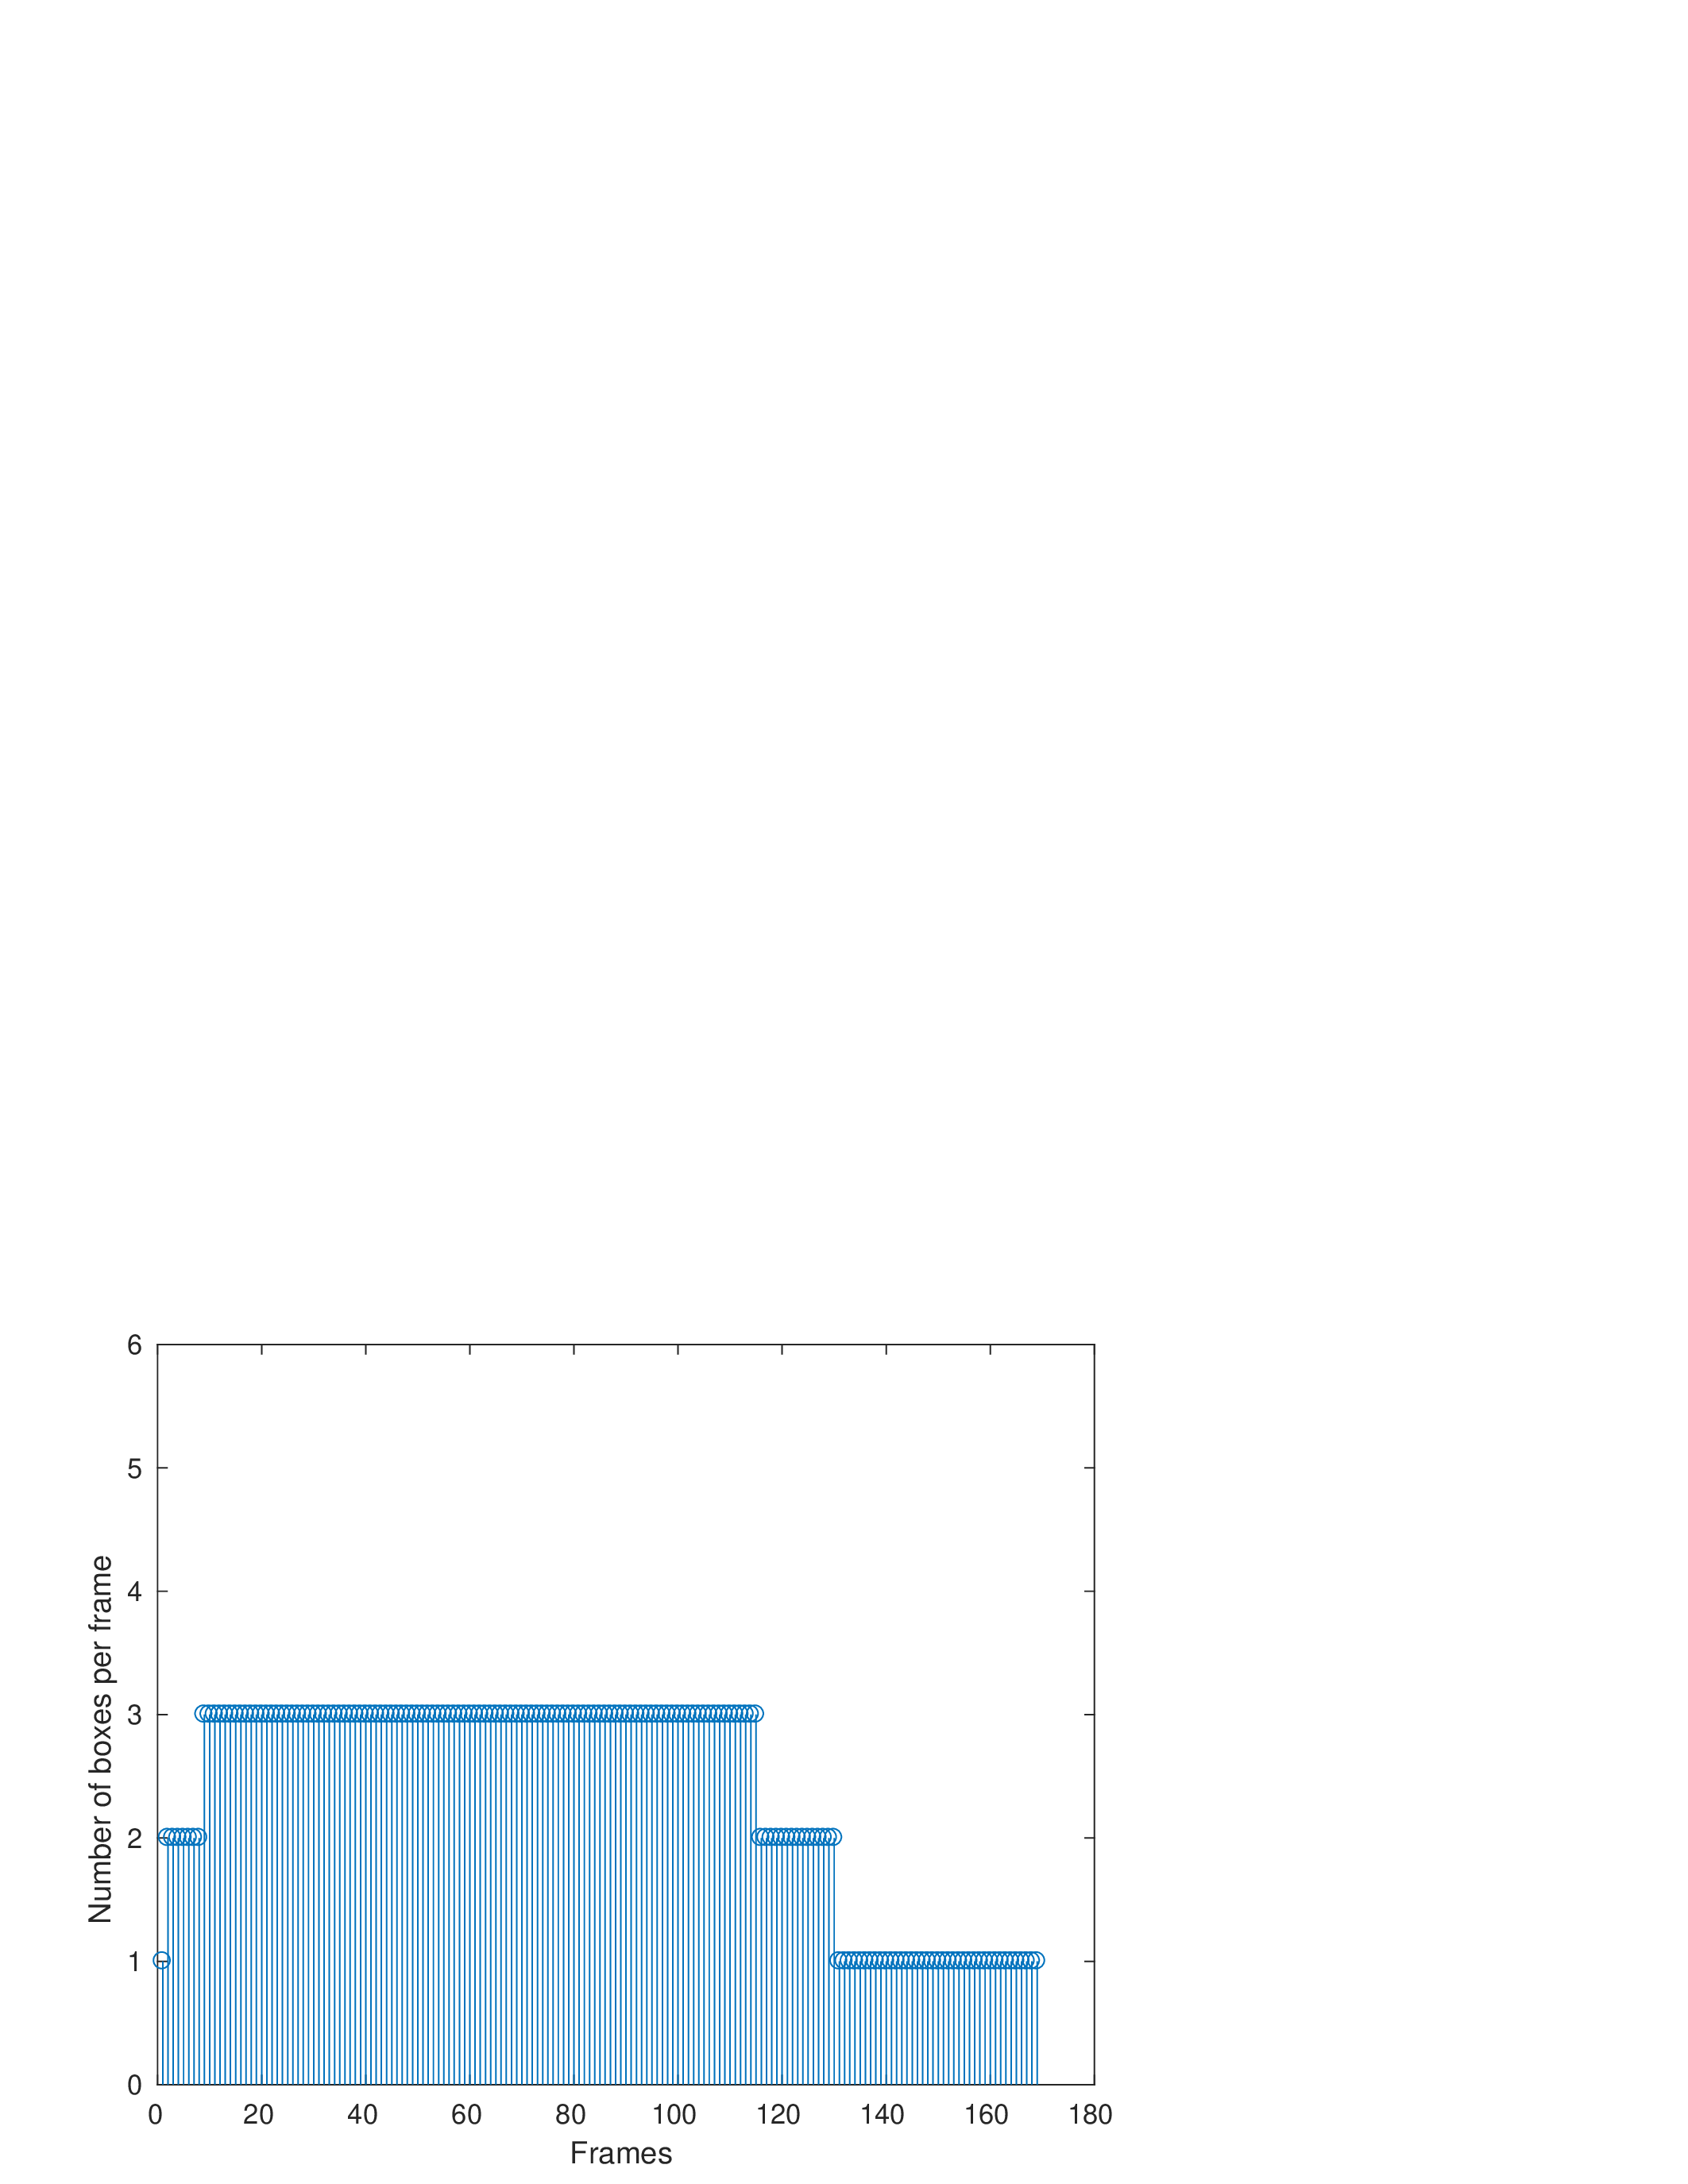}
       % \includegraphics[width=.28\linewidth]{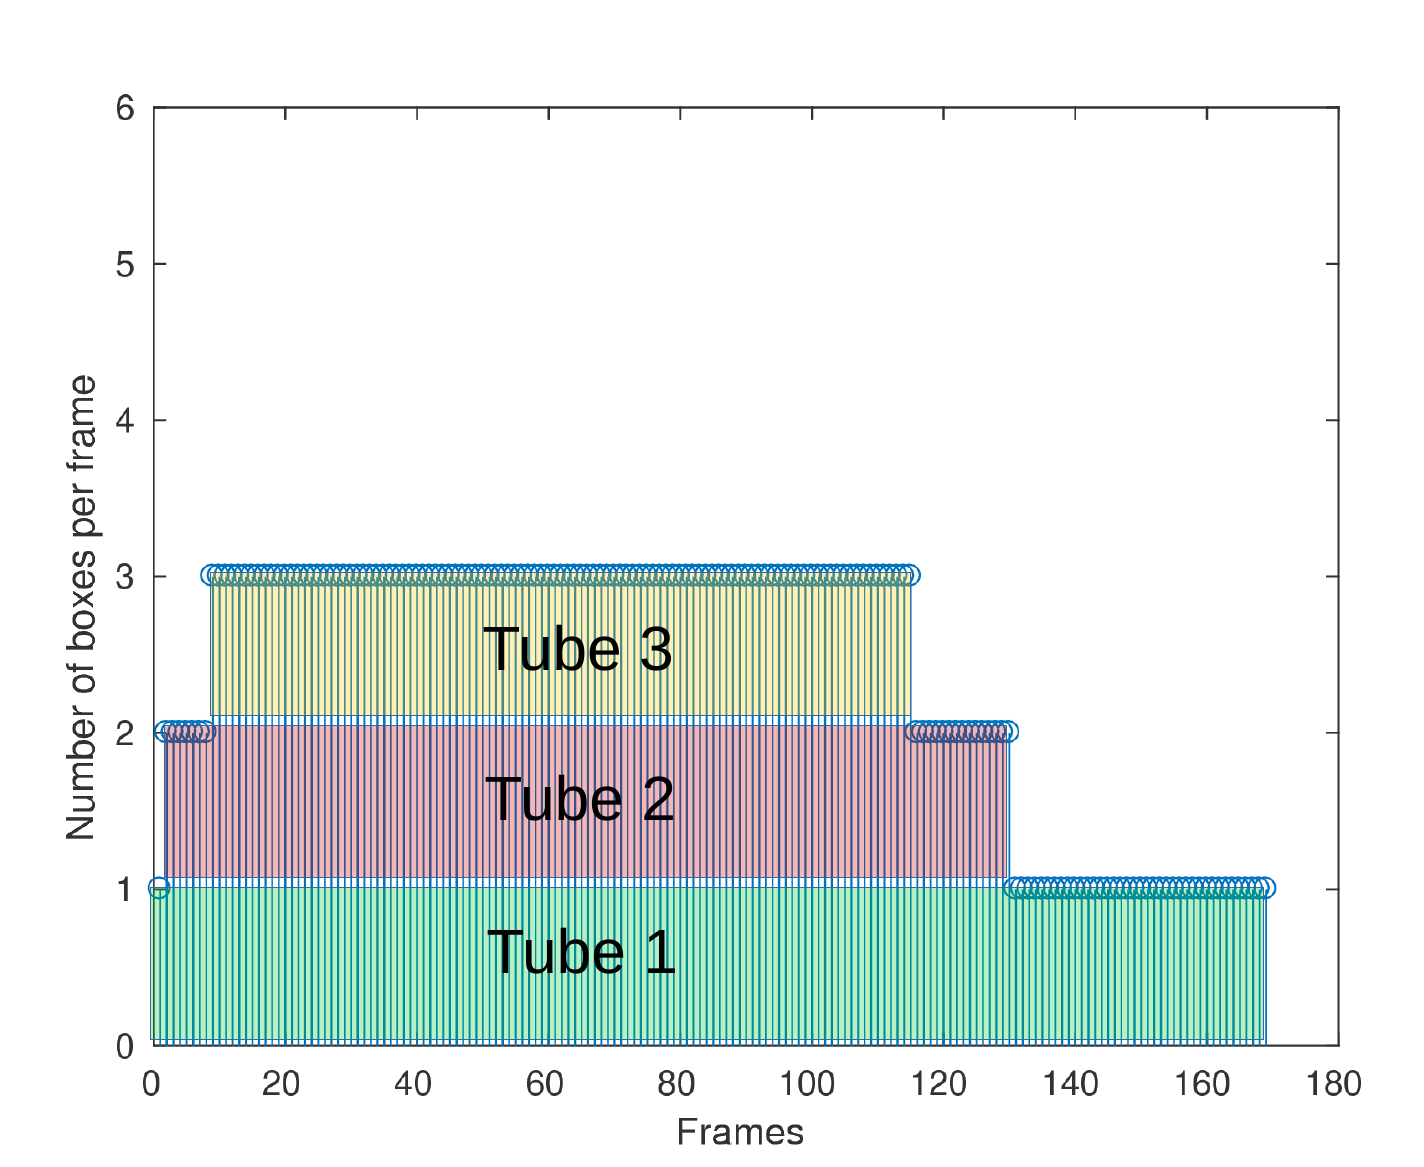}
         %\subcaption{}

    }  %\linebreak[1]
    \\
        \subfloat{%  
        \includegraphics[height=.4\linewidth,width=.75\linewidth]{images/smooth2.eps}

    }
    \\
        \subfloat{%  
        \includegraphics[height=.4\linewidth,width=.71\linewidth]{images/smooth2_1.pdf}

    }

    \caption{Preprocessing and extraction of the action tubes. The top figure shows the initial number of detected boxes per frame, $N_t$, the middle one shows the denoised version of it, $\hat{N}_t$ (section \ref{sec:prepr}), and the bottom figure shows the corresponding tube proposals. }
    \label{fig:preproc}
  %\vspace{-0.5cm}
  \end{figure}

 \begin{figure*}
 \centering
    \subfloat{%  
        \includegraphics[width=.16\linewidth]{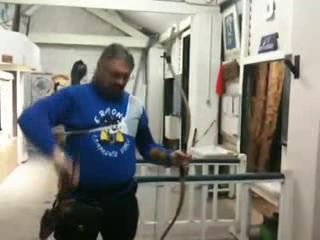}
        \includegraphics[width=.16\linewidth]{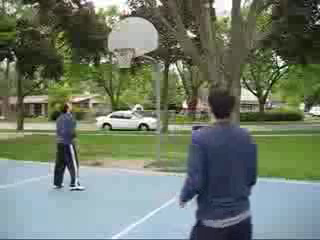}
        \includegraphics[width=.16\linewidth]{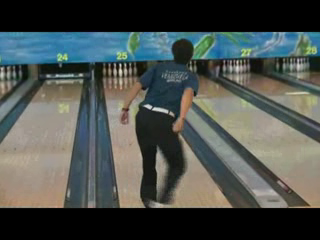}
        \includegraphics[width=.16\linewidth]{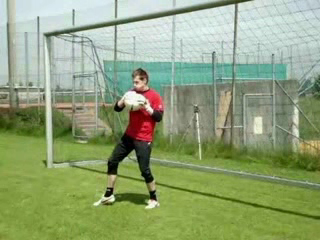}
        \includegraphics[width=.16\linewidth]{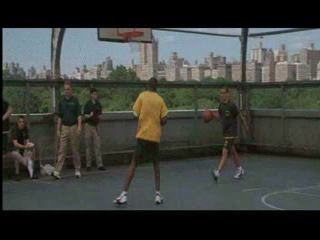}    \includegraphics[width=.16\linewidth]{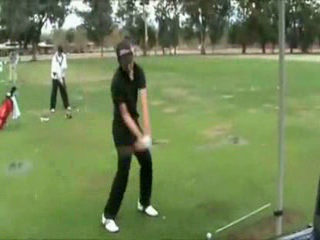}   
    }  %\linebreak[1]
    \\
    \subfloat{%
       \includegraphics[width=.16\linewidth]{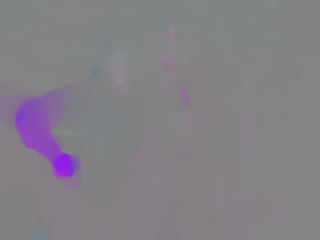}
        \includegraphics[width=.16\linewidth]{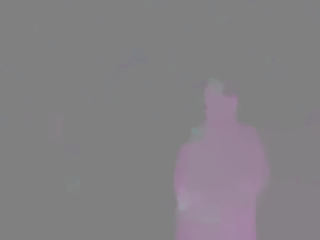}
        \includegraphics[width=.16\linewidth]{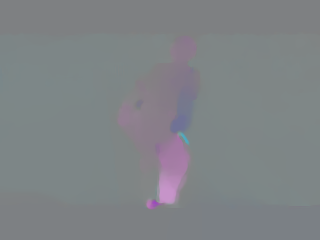}
        \includegraphics[width=.16\linewidth]{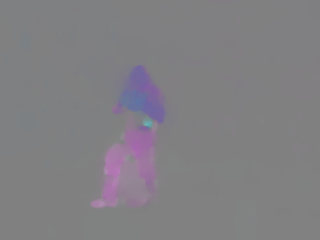}
        \includegraphics[width=.16\linewidth]{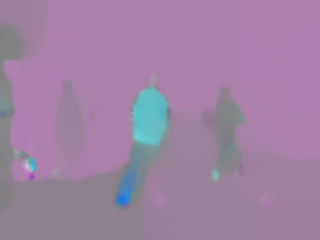}    \includegraphics[width=.16\linewidth]{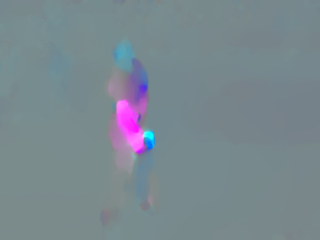}  
    } %\linebreak[1]
    \\
    \subfloat{%
        \includegraphics[width=.16\linewidth]{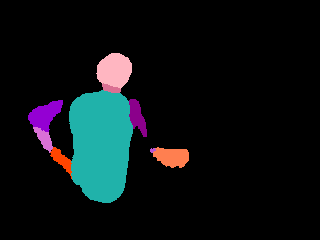}
        \includegraphics[width=.16\linewidth]{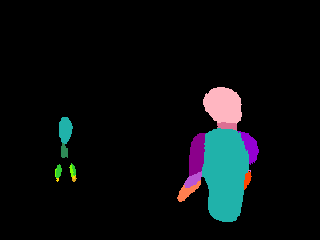}
        \includegraphics[width=.16\linewidth]{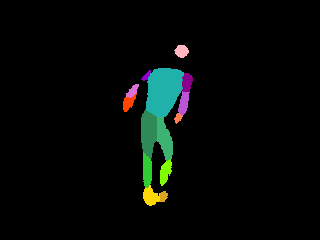}
        \includegraphics[width=.16\linewidth]{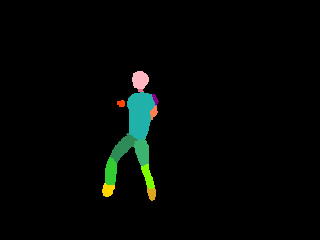}
        \includegraphics[width=.16\linewidth]{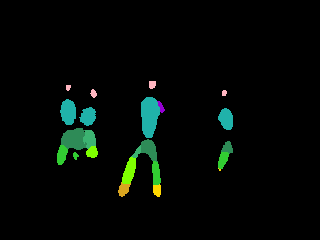}    \includegraphics[width=.16\linewidth]{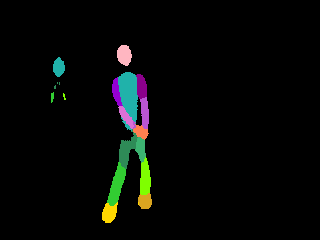}  
    } %\linebreak[1]

    \caption{Network inputs. \textbf{First row:} Raw image. \textbf{Second row:} Optical flow. 
\textbf{Third row:} Pose.}
    \label{fig:NetworkInputs1}
  %\vspace{-0.5cm}
  \end{figure*}
  
 \begin{figure*}
 \centering
    \subfloat{%  
        \includegraphics[width=.16\linewidth]{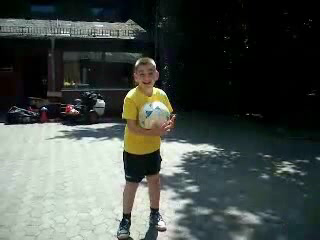}
        \includegraphics[width=.16\linewidth]{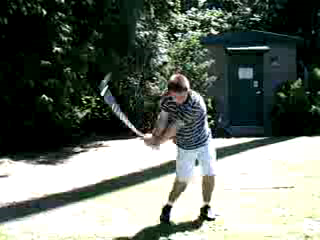}
        \includegraphics[width=.16\linewidth]{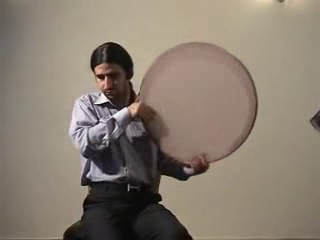}
        \includegraphics[width=.16\linewidth]{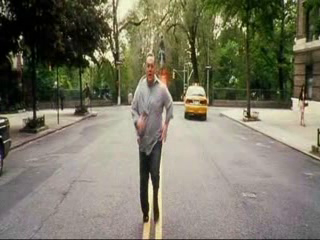}
        \includegraphics[width=.16\linewidth]{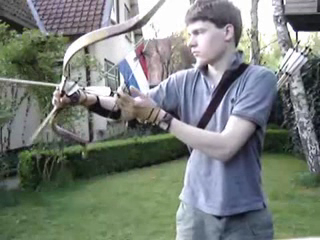}    \includegraphics[width=.16\linewidth]{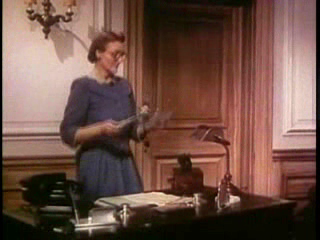}   
    }  %\linebreak[1]
    \\
    \subfloat{%
       \includegraphics[width=.16\linewidth]{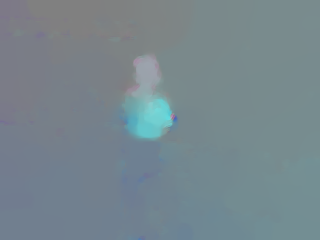}
        \includegraphics[width=.16\linewidth]{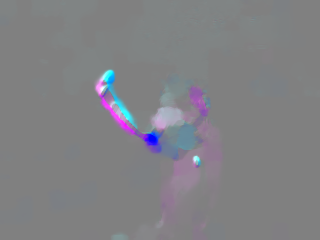}
        \includegraphics[width=.16\linewidth]{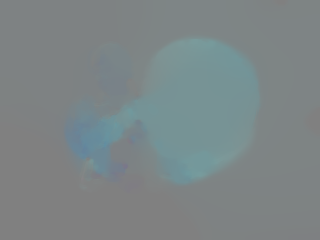}
        \includegraphics[width=.16\linewidth]{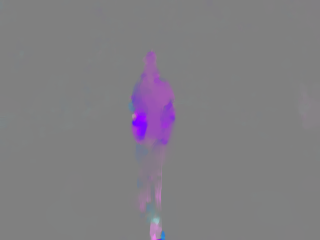}
        \includegraphics[width=.16\linewidth]{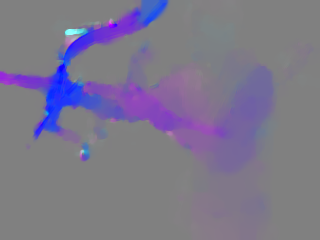}    \includegraphics[width=.16\linewidth]{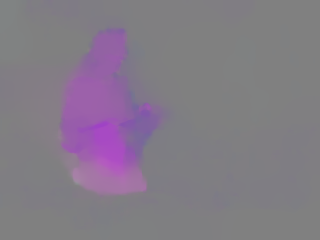}  
    } %\linebreak[1]
    \\
    \subfloat{%
        \includegraphics[width=.16\linewidth]{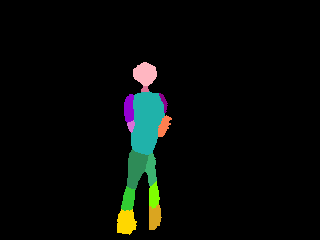}
        \includegraphics[width=.16\linewidth]{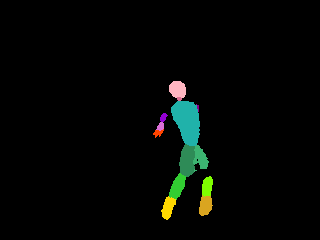}
        \includegraphics[width=.16\linewidth]{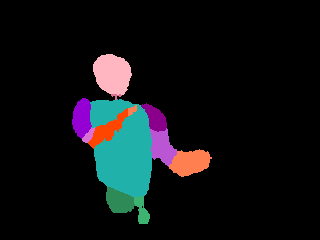}
        \includegraphics[width=.16\linewidth]{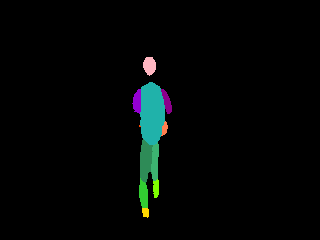}
        \includegraphics[width=.16\linewidth]{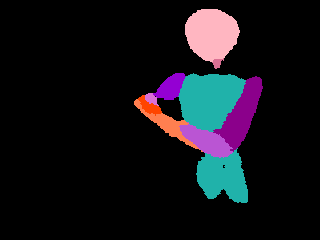}    \includegraphics[width=.16\linewidth]{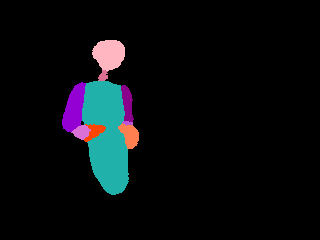}  
    } %\linebreak[1]

    \caption{Network inputs. \textbf{First row:} Raw image. \textbf{Second row:} Optical flow. 
\textbf{Third row:} Pose.}
    \label{fig:NetworkInputs2}
  %\vspace{-0.5cm}
  \end{figure*}

  %======================================================
  \section{Score aggregation}
For action classification, there are many approaches to aggregate features or scores obtained during the evaluations. In \cite{comp_pcnn}, they reported the performance of different feature aggregation schemes. 
We analyzed two different augmentation and three fusion methods to yield the final label for each video at test time. 

The two augmentation methods are (1) crop from the center of the frame, and horizontal flipping (\textbf{center-cropping}); (2) crop from the center and from 4 corners, and horizontal flipping (\textbf{fixed-cropping}). 
For fusion we used \textbf{mean}, \textbf{max}, and \textbf{majority voting} methods to calculate final scores.

In Table \ref{tab:scorefusions}, we provide the result of action recognition on all datasets with different score fusion and augmentation schemes. Like \cite{comp_tsn}, we observed that mean fusion in general provides better results than the other two fusion methods. In addition, fixed-cropping led to an increase of performance. 

Since actions can span various time intervals, we analyzed videos at multiple temporal scales. In all networks, the length of the input clips was 16 frames, but for \textbf{Net$_{16}$} we used a sampling rate of 1, for \textbf{Net$_{32}$} the sampling rate is 2, and \textbf{Net$_{W}$} refers to selecting 16 frames randomly from the entire video. We use the combined score for our multigrained action classification experiment in the main paper. A comparison of the single time scales is shown in Table \ref{tab:scorefusions}.

\begin{table*}
\centering
\begin{tabular}{|c|l|c|c|c|c|c|c|}
\hline
%\multicolumn{3}{|c|}{JHMDB} \\
%\hline
 \multirow{2}{*}{\textbf{Datasets}}&\multirow{2}{*}{\textbf{Networks}} &\multicolumn{3}{c|}{\textbf{Center-Cropping}}&\multicolumn{3}{c|}{\textbf{Fixed-Cropping}}\\
 \cline{3-8}
 &  & \textbf{mean} & \textbf{max} & \textbf{MajorityVoting}& \textbf{mean} & \textbf{max} & \textbf{MajorityVoting} \\ \hline \hline

\multirow{3}{*}{UCF101} & Net_{16}  & 87.9\% & 87.6\% & 85.4\% & 90.4\% & 89.8\% & 89.7\% \\ 
                        & Net_{32}  & 87.9\% & 87.3\% & 86.9\% & 90.3\% & 89.7\% & 89.5\% \\ 
                        & Net_{W}   & 86.6\% & 86.8\% & 86.4\% & 89.6\% & 89.0\% & 88.8\% \\  \hline 
\multirow{3}{*}{HMDB51}  
                        & Net_{16}  & 57.6\% & 56.7\% & 56.8\% & 62.1\% & 60.1\% & 60.3\%\\ 
                        & Net_{32}  & 58.7\% & 59.3\% & 58.2\% & 62.8\% & 61.1\% & 61.5\% \\ 
                        & Net_{W}   & 62.6\% & 62.3\% & 62.0\% & 66.0\% & 65.9\% & 65.5\%     \\ \hline
\multirow{1}{*}{J-HMDB}
                        & Net_{16}  & 81.7\% & 76.1\% & 78.4\% & 79.1\% & 78.7\% & 74.3\% \\
 \hline
\multirow{1}{*}{NTU RGB+D \cite{comp_ntu_cvpr}} 
                        & Net_{16} & 80.1\% & 77.2\%  & 79.6\% & 80.8\% & 80.3\% & 76.6\% \\
 \hline
 %& Ours (baseline) + SVM & 74.6\% \\
 %& Ours (chained) + SVM & 78.0\% \\ \hline
\end{tabular}
\caption{Comparison of the performance of different score fusion and augmentation methods for action recognition on the UCF101, HMDB51, and J-HMDB datasets (split 1) and NTU RGB+D dataset (Cross subject). }
\label{tab:scorefusions}
\end{table*}

%%%%%%%%% BODY TEXT
\section{Action Detection}
\subsection{Spatial localization}
We obtain human body part segmentations by our pose estimation network and simply generate the bounding box from the human body parts. 
We report quantitative results on J-HMDB dataset in the main paper. Here we additionally show some qualitative results on J-HMDB and UCF101 in Figure \ref{fig:qual_detect}.

 \begin{figure*}
 \centering
    \subfloat{%  
        \includegraphics[width=.16\linewidth]{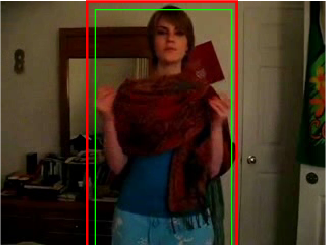}
        \includegraphics[width=.16\linewidth]{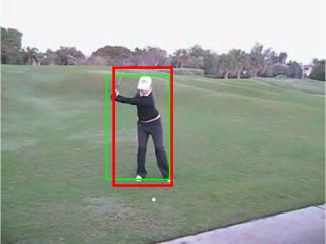}
        \includegraphics[width=.16\linewidth]{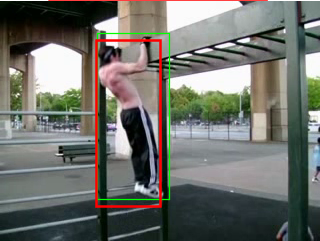}
        \includegraphics[width=.16\linewidth]{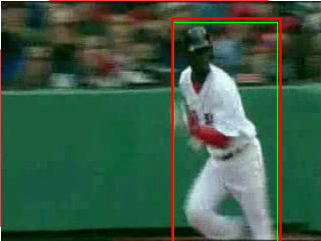}
        \includegraphics[width=.16\linewidth]{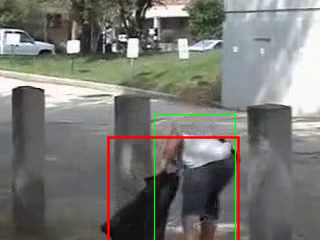}  
        \includegraphics[width=.16\linewidth]{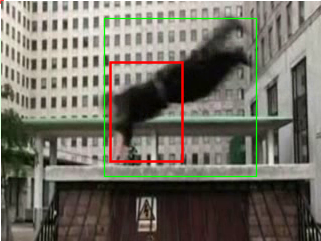}   
    }  %\linebreak[1]
    
        \subfloat{%  
        \includegraphics[width=.16\linewidth]{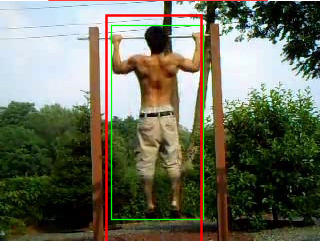}
        \includegraphics[width=.16\linewidth]{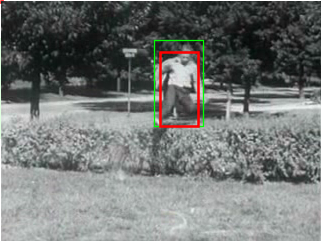}
        \includegraphics[width=.16\linewidth]{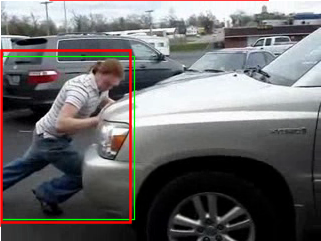}
        \includegraphics[width=.16\linewidth]{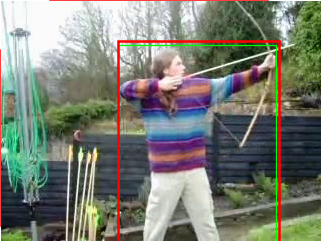}
        \includegraphics[width=.16\linewidth]{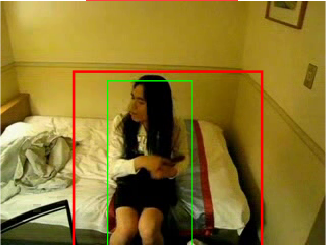}    \includegraphics[width=.16\linewidth]{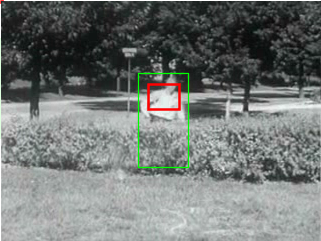}   
    }  %\linebreak[1]
    
    \subfloat{%
        \includegraphics[width=.16\linewidth]{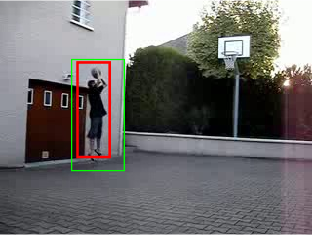}
        \includegraphics[width=.16\linewidth]{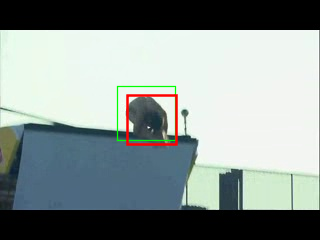}
        \includegraphics[width=.16\linewidth]{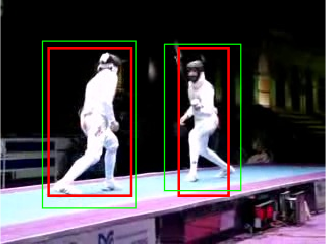}
        \includegraphics[width=.16\linewidth]{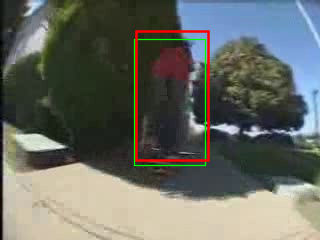}
        \includegraphics[width=.16\linewidth]{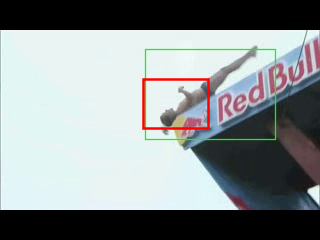}  
        \includegraphics[width=.16\linewidth]{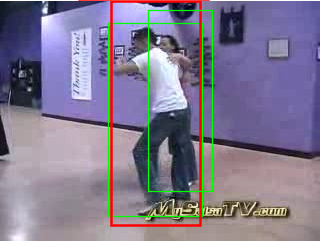}  
    } %\linebreak[1] 
    \\
    \subfloat{%
        \includegraphics[width=.16\linewidth]{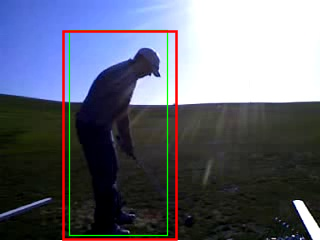}
        \includegraphics[width=.16\linewidth]{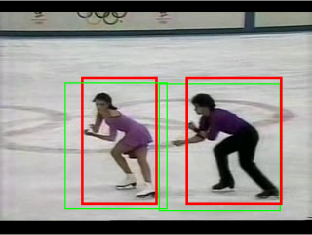}
        \includegraphics[width=.16\linewidth]{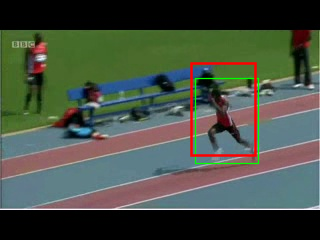}
        \includegraphics[width=.16\linewidth]{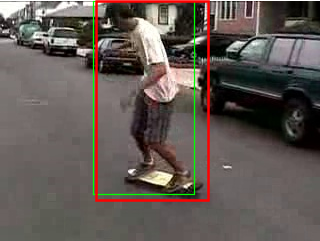}
        \includegraphics[width=.16\linewidth]{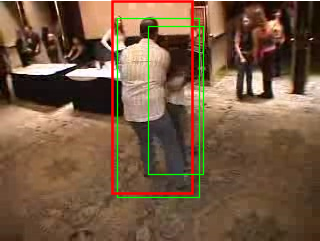}    
        \includegraphics[width=.16\linewidth]{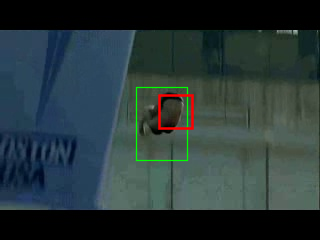}  
    } %\linebreak[1]

    \caption{Qualitative results. The first
two rows correspond to detections on J-HMDB, the last ones on
UCF101. In each row, the last two columns shows the failed detection examples.  Ground truth bounding boxes are shown in green and
detections in red.}
    \label{fig:qual_detect}
  %\vspace{-0.5cm}
  \end{figure*}
  
\subsection{Spatio-temporal localization}

%--------------
\paragraph{Preprocessing}
\label{sec:prepr}
To mitigate the effect of noise from our detections (false human detections, missed human instances), we define the \emph{expected} number of boxes per each frame of the input video clip, based on the expected arrangement of the action-tubes. 
To this end, we define signal $N_t$, which represents the number of detected boxes versus frame number -- Figure~\ref{fig:preproc}.
Then we use a median filter of size 80 to obtain a smoother version of it, $\hat{N}_t$, as in Figure~\ref{fig:preproc}. 
The final number of expected boxes in each frame is computed as follows:
\begin{equation}
 N^*_t=\max{(N_t,\hat{N}_t)}
\end{equation}

\noindent Whenever $N_t<N^*_t$ we simply create duplicate boxes from the box with the biggest size in that frame. Possible extra boxes are left intact and the box tracking algorithm that follows, picks the appropriate ones to use.

%--------------
\paragraph{Iterative Extraction of Action Tubes}
We define action tube proposals in the input video, based on the continuous regions in $\hat{N}_t$ -- Figure~\ref{fig:preproc}. We start with the longest one, trim the video to include only its time-span, and feed the obtained video clip to the Box Tracking algorithm. The output is a single action tube in the specified time span, and the detected boxes are removed from the initial set.
Tube proposals of length less than 5 frames are ignored. We repeat these steps until no tube proposal is left.

%--------------
\paragraph{Box Tracking}
For each action $a$ in the video, we define the following optimization function:
\begin{equation}
\begin{align}
 \overline{B}_a= arg\max_{\overline{B}} \frac{1}{T} \sum_{t=t_e}^{t_s}S_a(b_t,b_{t+1})
\end{align}
\end{equation}
\noindent where $\overline{B}_a=[b_s,b_{s+1},...,b_e]$ is the sequence of linked detection boxes from frame $s$ to frame $e$, $T$ is the tube length and $S_a(b_t,b_{t+1})$ denotes the linking score between consecutive frames $t$ and $t+1$. In our framework, $S_a$ is the IoU overlap of the two detection boxes. We can find the path by solving the above optimization problem using Viterbi algorithm \cite{comp_actiontubes}. After finding the optimal path, we remove all boxes in $\overline{B}_a$ and repeat this for finding the next optimal path until the set of boxes is empty.

%--------------
\paragraph{Temporal Actionness Score}
As discussed in section $5.3$ of the main paper, we calculate an actionness score for the frames of each video, based on the network outputs. More specifically, we leverage the scores obtained from the three streams as follows:

\begin{equation}
 s_{total} = (s_{pose})^2 \cdot (s_{rgb})^{1/3} \cdot (s_{flow})^{1/3}
\end{equation}

\noindent where $s_{pose}$, $s_{rgb}$ and $s_{flow}$ are the outputs of the softmax layers.
We sum the per-frame scores over each single tube, to assign an overall actionness score to each tube.
